# Supplementary material for: Simulation and Data Assimilation in an Idealized Coupled Atmosphere-Ocean-Sea Ice Floe Model with Cloud Effects
Source: arXiv:2410.23138 source file (2024-10-30)
Supplement: Supplementary file 1 [file draft_section_appendix.tex]

\appendix

%%%%%%%%%%%%%%%%%%%%%%%%%%%%%%%%%%%%%%%%%%%

\section{Ensemble transform Kalman Filters}
\subsection{Algorithm}
\begin{enumerate}
    \item \textbf{Initialization:}
    \begin{itemize}
        \item Initialize ensemble of state estimates $\{ \mathbf{x}_0^{(i)} \}_{i=1}^{N}$, where $N$ is the number of ensemble members.
        \item Estimate initial ensemble mean $\overline{\mathbf{x}}_0$ and perturbations $\mathbf{X}_0$.
    \end{itemize}
    
    \item \textbf{Forecast Step:}
    \begin{itemize}
        \item Propagate each ensemble member through the model to obtain forecasted states at time $t$:
        \[ \mathbf{x}_t^{f,(i)} = \mathcal{M}(\mathbf{x}_{t-1}^{(i)}) \]
        where $\mathcal{M}$ is the model operator.
        \item Calculate forecast ensemble mean $\overline{\mathbf{x}}_t^f$ and perturbations $\mathbf{X}_t^f$.
    \end{itemize}
    
    \item \textbf{Analysis Step:}
    \begin{itemize}
        \item Obtain observations $\mathbf{y}_t$ and compute observation perturbations $\mathbf{Y}_t$.
        \textbf{Note the observations $\mathbf{y}_t$ may not necessarily be the same in variables because the observations of floes may be different based on the cloud covering of atmosphere.}
        \item Compute the Kalman gain matrix $\mathbf{K}_t$ and the transformed ensemble perturbations $\mathbf{T}_t$:
        \[ \mathbf{K}_t = \mathbf{X}_t^f \mathbf{Y}_t^T (\mathbf{Y}_t \mathbf{Y}_t^T + \frac{\mathbf{R}}{N-1})^{-1} \]
        \[ \mathbf{T}_t = (\mathbf{I} + \mathbf{K}_t \mathbf{H} \mathbf{X}_t^f)^{-1/2} \]
        where $\mathbf{H}$ is the observation operator and $\mathbf{R}$ is the observation error covariance, $\mathbf{I}$ is the identity matrix.
        \item Update each ensemble member:
        \[ \mathbf{x}_t^{a,(i)} = \overline{\mathbf{x}}_t^f + \mathbf{X}_t^f \mathbf{T}_t^{(i)} \]
        where $\mathbf{x}_t^{a,(i)}$ represents the analyzed ensemble members.
    \end{itemize}
\end{enumerate}
\subsubsection{Matrix Formulation of the algorithm}
For a $2n\times 2n$ grid point observational data of atmospheric streamfucntion, we first transfer it into the $2n\times 2n$ Fourier modes and extract $2n^2-2$ complex modes $u_j(t_k),j=1,\cdots,2n^2-2$ and $3$ real modes, $v_j(t_k),j=1,2,3$. Then we have the following observed state variables for streamfunction:
\begin{align}
 U^a_1(t_k) = 
    \begin{bmatrix}
        v_1(t_k)\\
        v_2(t_k)\\
        v_3(t_k)\\
        Re(u_1(t_k))\\
        Re(u_2(t_k))\\
        \vdots\\
        Re(u_{2n^2-2}(t_k))\\
                Im(u_1(t_k))\\
        Im(u_2(t_k))\\
        \vdots\\
        Im(u_{2n^2-2}(t_k))\\
    \end{bmatrix}
    \in\mathbf{R}^{4n^2-1}
\end{align}
We also have the trajectories, $(x,y)$ coordinates, for $L$ different floes:
\begin{align}
    U_x(t_k) = \begin{bmatrix}
        x_1(t_k)\\
        x_2(t_k)\\
        \vdots\\
        x_L(t_k)\\
    \end{bmatrix}
        \in\mathbf{R}^{L}
    ,\qquad
        U_y(t_k) = \begin{bmatrix}
        y_1(t_k)\\
        y_2(t_k)\\
        \vdots\\
        y_L(t_k)\\
    \end{bmatrix}
            \in\mathbf{R}^{L}
\end{align}
Therefore, suppose we have observation about the surface atmospheric wind and the locations of the floes, we will have the observed state variable $U$ at each observation time $t_k$ which yields:
\begin{align}
    U(t_k) = U^a_1(t_k)\oplus U^a_2(t_k)\oplus U^o(t_k)\oplus U_x(t_k) \oplus U_y(t_k) \in\mathbf{R}^{3(4n^2-1)+2L}
\end{align}
Suppose the following:
\begin{itemize}
    \item The observations of ice floes' trajectories are affected by the cloud and not all ice floes are observed each time, thus $g$ is the observational operator $g_m$ changes at each time step $t_m$.
    \item The observations of observed variables differs each time step, i.e., the size of ${\bf v}_{obs}(t_m)$ does not equal to the size of $ {\bf v}_{obs}$
\end{itemize}
Then at $m$th observation time, we perform the ETKF:
\begin{enumerate}
    \item Put the Fourier transform of ensemble streamfunction $\widehat{\psi}_1^{a,k}(t_m)$, $\widehat{\psi}_2^{a,k}(t_m)$,$\widehat{\psi}^{o,k}(t_m)$ and location $(x^{k}(t_m),y^{k}(t_m)),k=1,\cdots,K$ in to the observed state variable vector form:
\begin{align}
    U^{(m)}\in \mathbf{R}^{N\times K}, \text{where } N =  3(4n^2-1)+2L. 
\end{align}

\item Calculate the mean of ensemble matrix $U^{(m)}$, i.e.,
\begin{align}
    \bar{U}^{(m)} = \frac{1}{K} \sum_{k=1}^K U_{\cdot k}^{(m)}
\end{align}
\item Calculate the perturbation matrix, $\widetilde U^{(m)}$ and $\widetilde v^{(m)}$, where 
\begin{align}
    &\widetilde{U}_{\cdot k}^{(m)}= U_{\cdot k}^{(m)}-\bar{U}^{(m)}, k=1,\cdots,K. 
    \\
    & \widetilde{V}_{\cdot k}^{(m)}= g_m(U_{\cdot k}^{(m)})-\bar{g_m(U)}^{(m)}, k=1,\cdots,K. 
\end{align}
where $g_m$ is the observational operator.
\textbf{The observational operator changes every time since the floes are observed differently at each time step.}

    % \item Form the $U^{(m)}$, $V^{(m)}$ matrices, where $U^{(m)}\in\mathbb{R}^{N\times K}$ is the perturbation matrix with respect to ensemble mean of ensemble size $K$ for all $N$ variables, $V^{(m)}\in\mathbb{R}^{N_{obs}\times K}$ is the perturbation matrix with respect to ensemble mean of ensemble size $K$ for  $N_{obs}$ observational variables. 
    \item Calculate the $J$ matrix
    \begin{align}
        J = \frac{K-1}{1+r}\mathcal{I}+ ( \widetilde V^{(m)})^T (R^o)^{-1}   \widetilde V^{(m)}
    \end{align}
    where $K$ is the ensemble size, $r$ is the inflation rate, and, $R^o$ is covariance matrix of observational noise which is pre-assigned. 
    \item Calculate the eigenvalue and eigen-vector for $\frac{J+J'}{2}$
    such that
    \begin{align}
        J = {\bf X}\Gamma {\bf X}^T
    \end{align}
    \item Calculate 
    \begin{align}
        x = J^{-1} {(V^{(m)})}^T (R^o)^{-1} ({\bf v}_{obs}^{m} - \bar{U}^{(m)})
    \end{align}
    \item 
    Calculate the posterior mean for {\bf u}
    \begin{align}
        \overline{U}_{m|m} = \overline{U}^{(m)} +  \widetilde U^{(m)}x
    \end{align}
    \item Calculate the transformation matrix
    \begin{align}
        T = \sqrt{K-1} {\bf X}\Gamma^{-1/2}{\bf X}^T 
    \end{align}
    \item Update the posterior perturbation matrix
    \begin{align}
        \widetilde U_{m|m}^{(m)} =  \widetilde U^{(m)} T.
    \end{align}
    \item Update the posterior matrix:
    \begin{align}
         U_{m|m}^{(m)} = \overline{U}_{m|m} + \widetilde U_{m|m}^{(m)} .
    \end{align}
\end{enumerate}
\begin{remark}
    For every time updating the \textbf{prior} or \textbf{posterior} state variables of trajectories, we must consider the double periodic boundary conditions by setting the constraints:
    \begin{align}
        0<x<L, 0<y<L
    \end{align}
    where $L$ is the square domain length.
\end{remark}
